# Supplementary material for: Diurnal and Seasonal Mapping of Martian Ices With EMIRS
Source: arXiv:2303.08328 source file (2023-06-27)
Supplement: Supplementary file 1 [file stcherbinine_GRL2023_EMIRS_ice_revisions1_SI.pdf]

# Supporting Information for ”Diurnal and Seasonal Mapping of Martian Ices with EMIRS”

DOI: 10.1002/2023GL103629

Aurélien Stcherbinine<sup>1</sup>, Christopher S. Edwards<sup>1</sup>, Michael D. Smith<sup>2</sup>,  
Michael J. Wolff<sup>3</sup>, Christopher Haberle<sup>1</sup>, Eman Al Tunaiji<sup>4</sup>, Nathan M.  
Smith<sup>1</sup>, Kezman Saboi<sup>1</sup>, Saadat Anwar<sup>5</sup>, Lucas Lange<sup>6</sup>, Philip R.  
Christensen<sup>5</sup>

<sup>1</sup>Department of Astronomy and Planetary Science, Northern Arizona University, Flagstaff, AZ, USA

<sup>2</sup>NASA Goddard Space Flight Center, Greenbelt, MD, USA

<sup>3</sup>Space Science Institute, Boulder, CO, USA

<sup>4</sup>Mohammed Bin Rashid Space Centre, Dubai, UAE

<sup>5</sup>School of Earth and Space Exploration, Arizona State University, Tempe, AZ, USA

<sup>6</sup>Laboratoire de Météorologie Dynamique (LMD/IPSL), Sorbonne Université, ENS, École Polytechnique, CNRS, Paris, France

## Contents of this file

### 1. Figure S1

---

Corresponding author: A. Stcherbinine, Department of Astronomy and Planetary Science,  
Northern Arizona University, Flagstaff, AZ 86001, USA. (aurelien.stcherbinine@nau.edu)

June 7, 2023, 5:19pm

**Introduction** This document provide a similar figure to Figure 1 but only for the CO<sub>2</sub> surface ice of the polar caps.

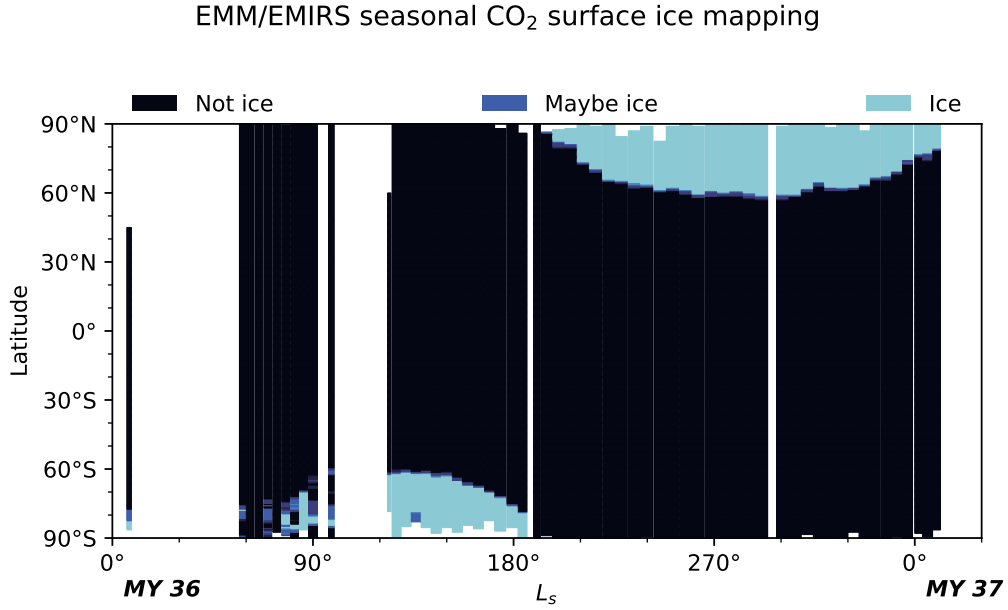

**Figure S1.** Seasonal variations of the latitudinal median extent of the Martian CO<sub>2</sub> polar caps from EMM/EMIRS retrievals. Only maps with a high-quality flag have been considered here. For every bin of 4 EMM orbits, the mapping of the CO<sub>2</sub> polar caps is computed as the median of the CO<sub>2</sub> detections over all local times from the local time CO<sub>2</sub> maps described in Section 2.3, considering only the areas with a high data density for every local time map.
